# Supplementary material for: SiPM array of Xenoscope, a full-scale DARWIN vertical demonstrator
Source: arXiv:2303.15300 source file (2023-03-27)
Supplement: Supplementary file 1 [file appendix.tex]

\appendix
\section{Readout electronics schematic}
\label{app:tilereadoutscheme}

\begin{figure}[!h]
    \centering
    \includegraphics[width=0.8\textheight, angle = -90]{Figures/tilecircuit.pdf}
    \caption{Circuit layout of the electronics readout for a tile module.}
\end{figure}
